# Supplementary material for: InfinityDrive: Breaking Time Limits in Driving World Models
Source: arXiv:2412.01522 source file (2024-12-04)
Supplement: Supplementary file 1 [file X_suppl.tex]

\clearpage
\setcounter{page}{1}

\setcounter{section}{0}
\setcounter{figure}{0}
\setcounter{table}{0}

\maketitlesupplementary

% \noindent\textbf{\LARGE Appendix}
% \tableofcontents
% \clearpage

% \section{Rationale}
% \label{sec:rationale}
% % 
% Having the supplementary compiled together with the main paper means that:
% % 
% \begin{itemize}
% \item The supplementary can back-reference sections of the main paper, for example, we can refer to \cref{sec:intro};
% \item The main paper can forward reference sub-sections within the supplementary explicitly (e.g. referring to a particular experiment); 
% \item When submitted to arXiv, the supplementary will already included at the end of the paper.
% \end{itemize}
% % 
% To split the supplementary pages from the main paper, you can use \href{https://support.apple.com/en-ca/guide/preview/prvw11793/mac#:~:text=Delete%20a%20page%20from%20a,or%20choose%20Edit%20%3E%20Delete).}{Preview (on macOS)}, \href{https://www.adobe.com/acrobat/how-to/delete-pages-from-pdf.html#:~:text=Choose%20%E2%80%9CTools%E2%80%9D%20%3E%20%E2%80%9COrganize,or%20pages%20from%20the%20file.}{Adobe Acrobat} (on all OSs), as well as \href{https://superuser.com/questions/517986/is-it-possible-to-delete-some-pages-of-a-pdf-document}{command line tools}.

\section{Additional Video Results}
%To better show the potential of InfinityDrive as a driving world model, we include video results of the proposed method in a demo webpage and we kindly ask the reader to refer to \textcolor{red}{\url{infinitydrive-webpage/page.html}} in the supplementary material package, best viewed in Chrome. \textcolor{red}{Please unzip the entire archive of supplementary materials before opening the webpage. It is recommended to use Windows and macOS systems instead of Linux.} These demo videos provide direct visual examples of InfinityDrive's capability of generating long-duration videos of high fidelity, high resolution, controllability, and diverse scenarios. 

\textbf{Firstly} in the website we include the long-duration results, where we show various videos of 150-second duration generated by InfinityDrive. \textbf{Secondly} to illustrate the controllability of InfinityDrive, we show generated videos in which the ego vehicle follows a input direction command such as \textit{Go Left/Right}. \textbf{Thirdly}, we include high-resolution generated videos, demonstrating the high-resolution generation ability of our methods. \textbf{In addition}, we include a parallel world section, where we show 24 different generated driving scenarios with the same initial condition(text or image) with different noise to provide examples of diverse outputs of our method. \textbf{Finally}, we conduct a comparison between the results of our method and other SOTA methods such as Vista\cite{vista}, to provide a direct visual example of our method's ability to handle corner cases of other methods.

\section{Preliminaries}
This section serves to introduce preliminary definitions and methods in diffusion models as contexts so we can better demonstrate our method in the main text. We briefly review some basic concepts needed to understand diffusion models and video DiT architecture.

\subsection{DDPM}
\noindent \textbf{Forward Diffusion Process:} The forward process gradually adds Gaussian noise to the data $x_0$ over time steps $T$:

\begin{equation}
q(x_t \mid x_{t-1}) = \mathcal{N}(x_t; \sqrt{\alpha_t} x_{t-1}, (1 - \alpha_t) I)
\end{equation}

where $\alpha_t$ is a variance schedule that controls the amount of noise added at each step.

\noindent \textbf{Marginal Distribution:} The marginal distribution of $x_t$ given $x_0$ can be expressed as:

\begin{equation}
q(x_t \mid x_0) = \mathcal{N}(x_t; \sqrt{\bar{\alpha}_t} x_0, (1 - \bar{\alpha}_t) I)
\end{equation}

where $\bar{\alpha}t = \prod{s=1}^t \alpha_s$.

\noindent \textbf{Reverse Diffusion Process:} The reverse process aims to denoise $x_t$ to recover $x_{t-1}$:

\begin{equation}
p_\theta(x_{t-1} \mid x_t) = \mathcal{N}(x_{t-1}; \mu_\theta(x_t, t), \Sigma_\theta(x_t, t))
\end{equation}

where $\mu_\theta$ and $\Sigma_\theta$ are parameterized by neural networks.

\noindent \textbf{Training Objective:} The model is trained to predict the added noise $\epsilon$ by minimizing the following loss function:

\begin{equation}
L = \mathbb{E}{x_0, \epsilon, t} \left[ \left| \epsilon - \epsilon\theta(x_t, t) \right|^2 \right]
\end{equation}

where $\epsilon \sim \mathcal{N}(0, I)$ and $t$ is uniformly sampled from ${1, \ldots, T}$.

\subsection{Video DiT Backbone}
\label{sec:dit}
We use OpenSora V1.1 as the backbone, but the VAE encoder and decoder are from the versions provided by SVD \cite{svd}. We found that this improves the temporal stability of the generated videos. The structure of the backbone is shown in Fig. \ref{fig:block}: the noisy real video is encoded by the VAE, passes through 28 identical STDiT blocks, and finally outputs the denoised video. To save computation, each block employs spatial and temporal separable attention operations and uses an AdaIN \cite{huang2017adain} modulator to inject the timestep embedding. Text and action are injected via cross-attention. Additionally, the timestep embedding is combined with embeddings of scalar values like FPS, video width, and height before being injected into the backbone; for simplicity, this operation is omitted in the figure.

In addition, we did not use OpenSora V1.2, even though this version offers better performance. This is because the VAE in V1.2 also compresses the temporal dimension, and we found that this temporal compression leads to significant detail loss when generating driving scenes. The likely reason is that driving scenarios typically involve fast motion, and compressing the temporal dimension results in the loss of too much information. How to achieve reasonable spatiotemporal compression for generating autonomous driving scenes might also be a topic worth further research.

\begin{figure}[t]
  \centering
  %\fbox{\rule{0pt}{2in} \rule{0.9\linewidth}{0pt}}
   \includegraphics[width=1.0\linewidth]{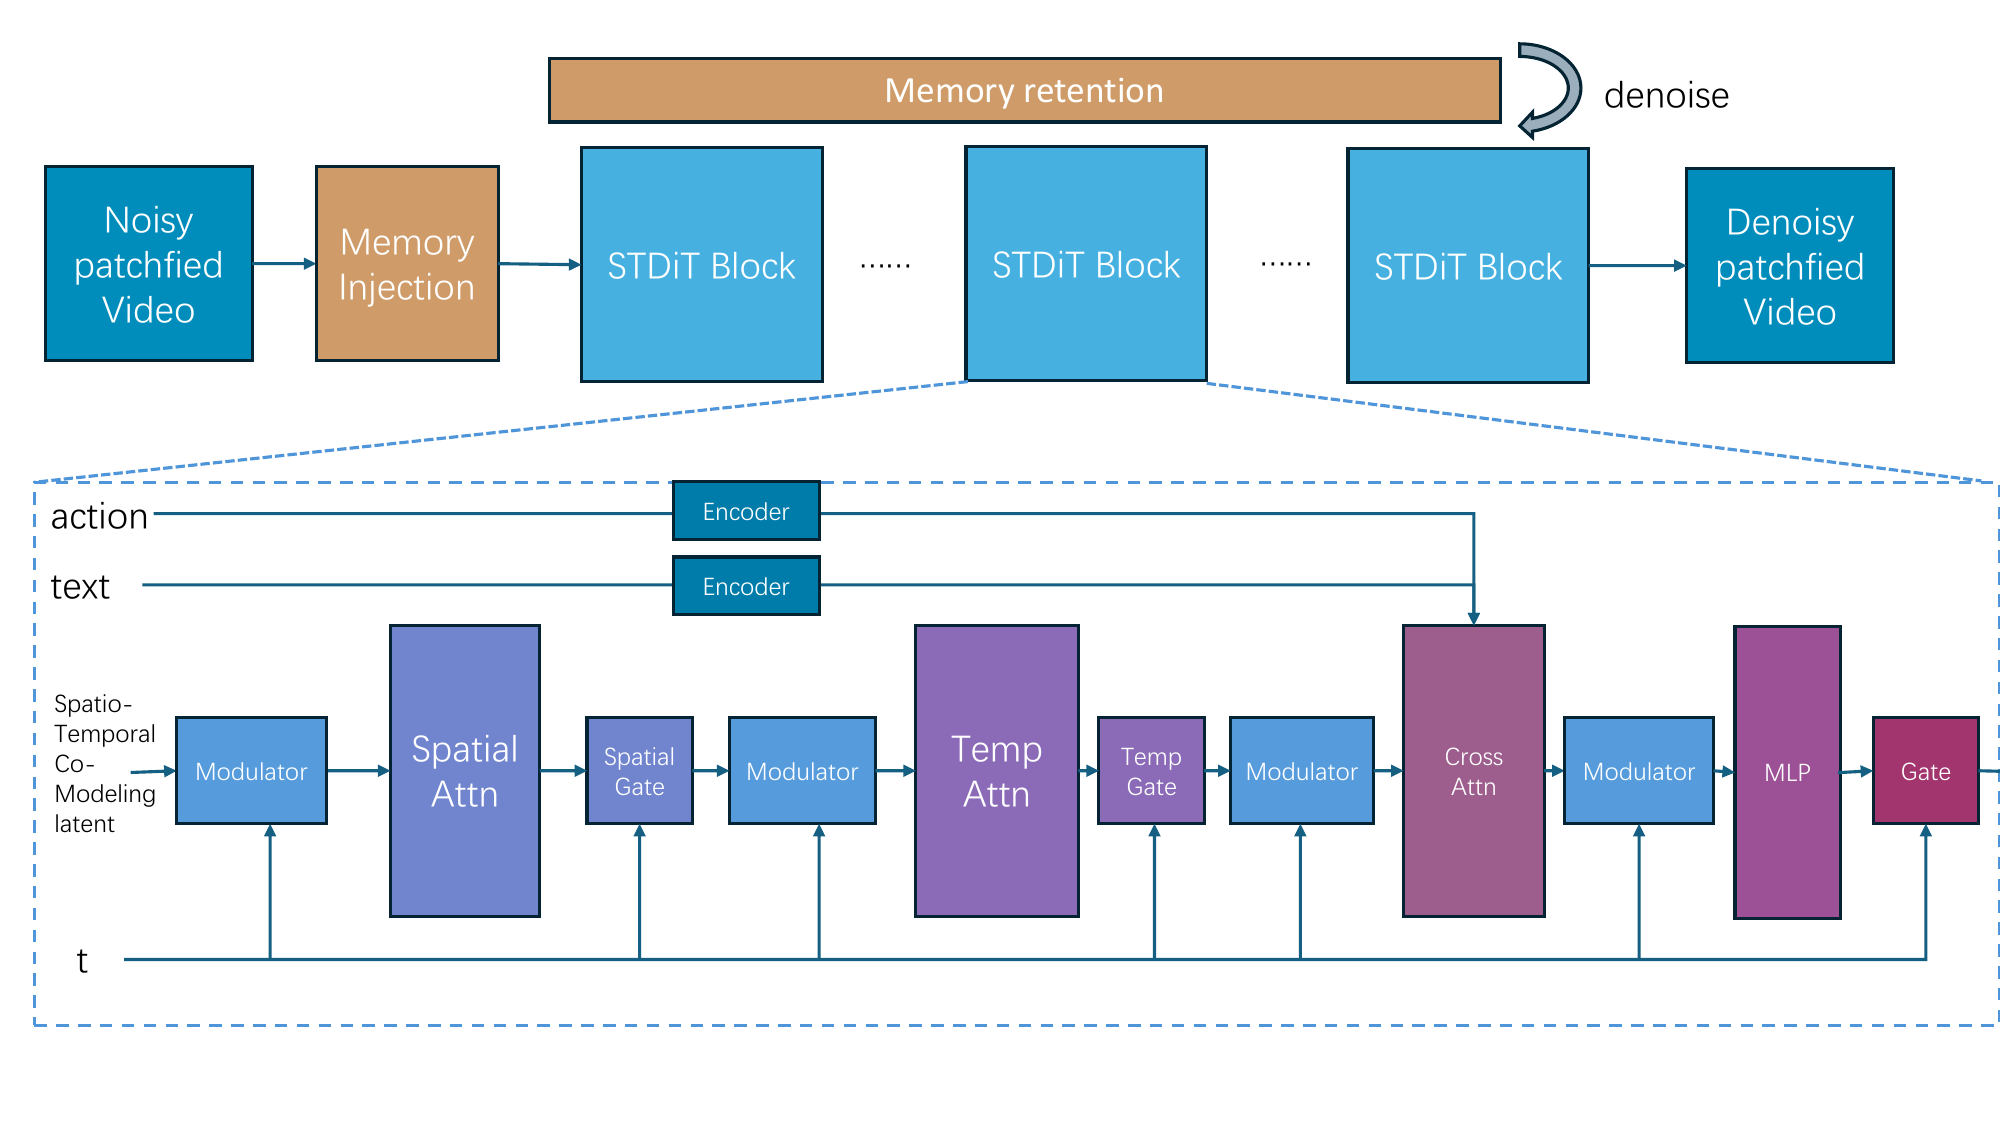}
   \caption{\textbf{Video Dit Backbone.} Please refer to the description in Sec. \ref{sec:dit} for more details.}
   \label{fig:block}
\end{figure}

\section{Additional Implementation Details}
\subsection{Datasets}
\label{sec: Datasets}
We use two representative datasets: OpenDV-2K\cite{genad} and nuScenes\cite{nuscenes}. To enhance diversity, we develop a re-captioning scheme for the nuScenes dataset and we provide examples of the generated captions in Tab~\ref{tab:prompt_examples}. OpenDV-2K and nuScenes are used as training datasets, and, following prior works, we conduct quantitative evaluations on the nuScenes evaluation dataset. 
% In addition, we validate our generalization validation on the Waymo dataset found in Appendix.
\subsection{Metrics}
\label{sec: Metrics}
Following previous work\cite{vista}, we adopt the Fr\'echet Inception Distance (FID)\cite{FID} to measure the quality of generated video frames, and the Fr\'echet Video Distance (FVD)\cite{fvd} as a measurement of temporal coherence. Additional metrics not covered in previous driving world models, aimed at better evaluating temporal consistency, background consistency, and diversity.

To better assess diversity and temporal consistency, we adopt the motion aware motion error (MAWE)\cite{streamingT2V} to capture the rich motion dynamics and consistency in synthesized videos. MAWE incorporates the mean warp error and the optical flow score to measure consistency while taking motion into consideration. In particular, for any given video the mean warp error calculates the averaged L2 distance between one frame and its warped following frame in pixel space in non-occluded regions. Furthermore, the optical flow score computes the average norm of optical flow vectors between any two consecutive frames, measuring the amount of motion in a given video. MAWE combines both measurements by dividing the mean warp error by the optical flow score and a coefficient which we set to be 9.5 as in the original paper\cite{streamingT2V}. The MAWE metric yields a low value when temporal consistency and rich motion dynamics are both present in the video.

In addition, we utilize the background consistency metric\cite{vbench}, which measures the consistency of the background scene. This metric calculates both the mean cosine similarity between CLIP\cite{clip} features of all consecutive frames, and the mean cosine similarity between CLIP features of first frame and all other frames, and then average the two similarities, measuring consistency across frames.

\begin{table*}[ht]
    \centering
    \begin{tabular}{|c|p{10cm}|} % Adjust the column width as needed
        \hline
        \multicolumn{1}{|c|}{\textbf{Input Video} (only show the first frame)} & \multicolumn{1}{c|}{\textbf{Generated Captions}} \\ \hline
        \raisebox{-\height}{\includegraphics[width=6cm]{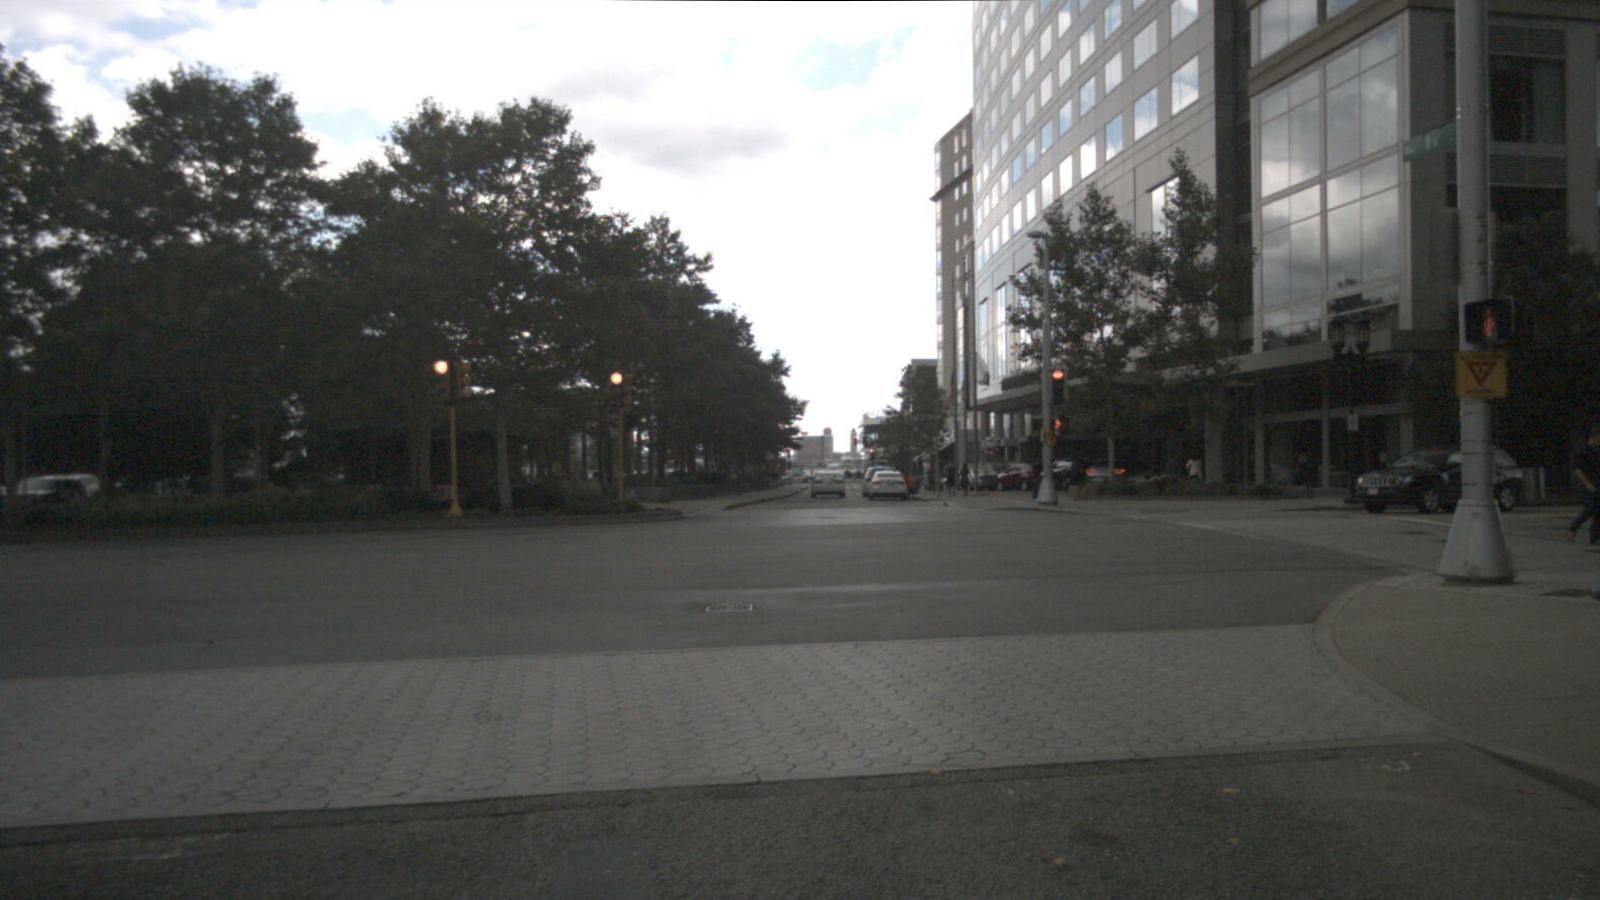}} & The video shows a city street at daytime with a car driving down the road. The street is empty, and there are no pedestrians visible. The lighting is dim, with streetlights illuminating the area. The car is the only vehicle in the scene, and there are no other vehicles or pedestrians that can potentially cross paths with the car. there is a traffic sign and a traffic light in the image. There are two lanes in the same direction. There are two lanes in the opposite direction. The ego vehicle is in the right lane. the ego vehicle is passing a junction in the city. The ego vehicle is moving, as it is seen driving down the street in the image. The ego vehicle is driving down the street, passing by a traffic light. \\ \hline
        \raisebox{-\height}{\includegraphics[width=6cm]{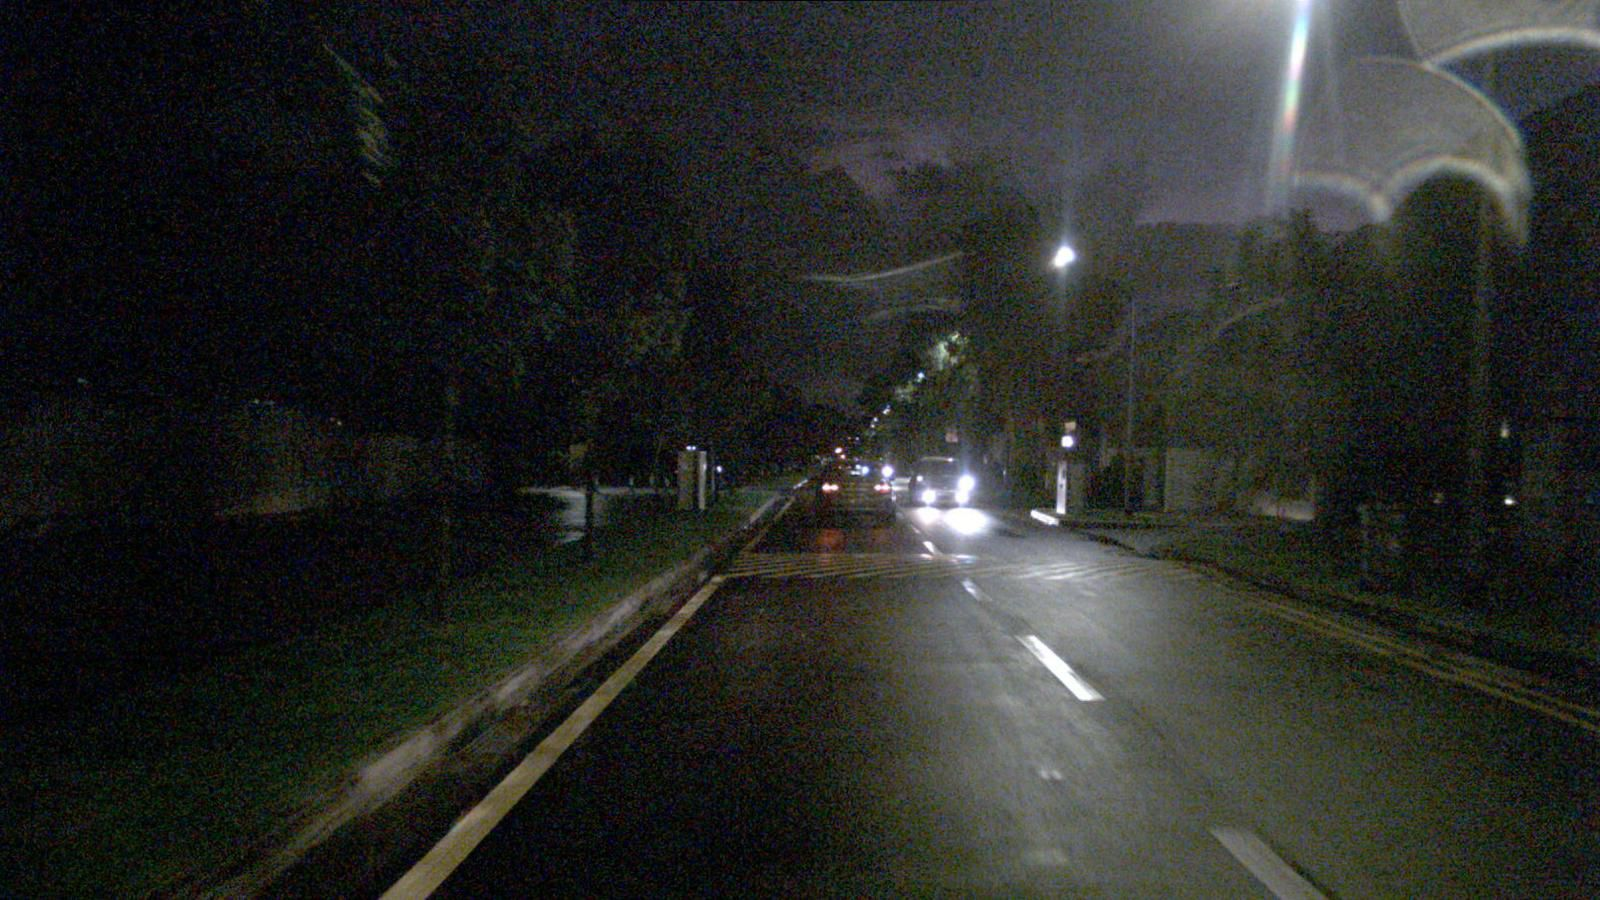}} & The video shows a dark street at night with a few cars and a truck driving down the road. The street is wet, which suggests that it has rained recently. The lighting is dim, with only a few streetlights and car headlights illuminating the area. The vehicles are moving at a moderate speed, and there is no indication of any sudden appearance of pedestrians. The ego vehicle is driving down the road, and the other vehicles are following behind it. The video captures the typical nighttime driving scenario in a city. there is a traffic sign on the side of the road. There are two lanes in the same direction. There are two lanes in the opposite direction. The ego vehicle is in the right lane. the ego vehicle is passing a junction in the video. The ego vehicle is moving, as it is seen driving down the street in the video. The ego vehicle is driving down the street, and it is seen in the foreground of the image. \\ \hline
        \raisebox{-\height}{\includegraphics[width=6cm]{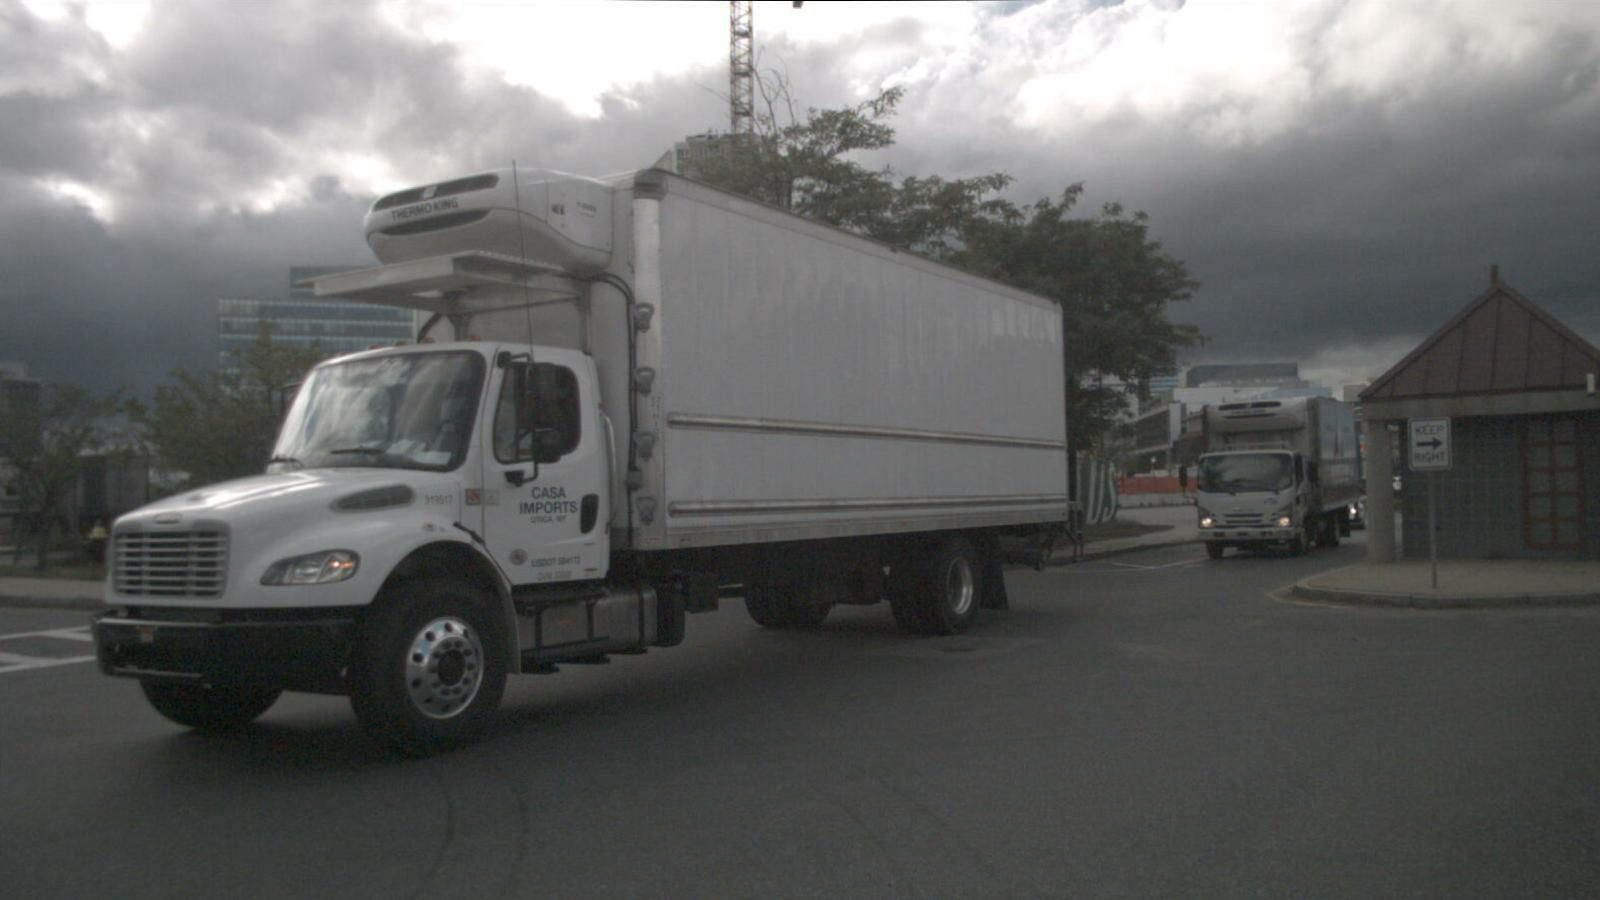}} & The video shows a cloudy day with a truck driving down a road. The truck is carrying a load of cargo, and there is a train visible in the background. The road is surrounded by trees, and there is a building nearby. The lighting is dim, with the sunlight being blocked by the clouds. The truck is the only vehicle in the video, and there are no pedestrians or other vehicles that can cross its path. There is a traffic sign visible in the image. There are two lanes in the same direction. There are two lanes in the opposite direction. The ego vehicle is in the left lane. the ego vehicle is passing a junction in the image. The ego vehicle is moving, as it is driving down the street. The ego vehicle is driving down the road, passing by a large truck. \\ \hline
    \end{tabular}
    \caption{Examples of generated captions, paired with the condition images of the corresponding driving scenarios with the frontal view.}
    \label{tab:prompt_examples}
\end{table*}

% \begin{table*}[ht]
% \centering
% \begin{tabular}{c|c|c|c|c|c}
% \hline
% Settings & Methods & FID$\downarrow$ & FVD$\downarrow$ & Background Consistency$\uparrow$ & MAWE$\downarrow$ \\ \hline
% \multirow{4}{*}{Long Term} 
% & SVD-XT~\cite{svd} & 42.99 & 275.08 & 0.92 & \textbf{1.06} \\ 
% & Vista~\cite{vista} & 34.61 & 234.60 & 0.92 & 1.78 \\ 
% & StreamingT2V-SVDXT~\cite{streamingT2V} & 181.22 & 1255.30 & \textbf{0.89} & 3.07 \\ 
% & Ours & \textbf{14.92} & \textbf{113.91} & 0.92 & 1.76 \\ \hline
% \end{tabular}
% \caption{Comparison of results for generating 100-frame long-duration videos on NuScenes. Our method demonstrates superior performance in terms of FID, FVD, highlighting its ability to generate high-quality, consistent long-duration driving scenarios.}
% \label{tab:long-term-comparison}
% \end{table*}

\begin{table*}[ht]
\centering
\begin{tabular}{|c|c|c|c|c|c|}
\hline
Metrics                                 & Methods      & All Frames      & Frame 0-40     & Frame 40-80     & Frame 80-120    \\ \hline
\multirow{4}{*}{FID}                    & SVD-xt       & 42.99           & 29.21          & 51.83           & 88.36           \\ %\cline{2-6} 
                                        & Vista        & 34.61           & 25.27          & 46.36           & 70.14           \\ %\cline{2-6} 
                                        & StreamingT2V & 181.22          & 127.16         & 217.70          & 242.91          \\ %\cline{2-6} 
                                        & Ours         & \textbf{14.93}  & \textbf{11.99} & \textbf{19.30}  & \textbf{19.53}  \\ \hline
\multirow{4}{*}{FVD}                    & SVD-xt       & 275.08          & 224.07         & 373.75          & 549.44          \\ %\cline{2-6} 
                                        & Vista        & 234.60          & 137.45         & 312.13          & 520.71          \\ %\cline{2-6} 
                                        & StreamingT2V & 1255.30         & 912.17         & 1717.02         & 2124.55         \\ %\cline{2-6} 
                                        & Ours         & \textbf{115.62} & \textbf{90.48} & \textbf{148.65} & \textbf{143.64} \\ \hline
\multirow{4}{*}{MAWE}                   & SVD-xt       & \textbf{1.06}   & \textbf{0.52}  & \textbf{0.71}   & 1.92            \\ %\cline{2-6} 
                                        & Vista        & 1.78            & 1.51           & 2.21            & 1.59            \\ %\cline{2-6} 
                                        & StreamingT2V & 3.07            & 2.51           & 2.94            & 3.77            \\ %\cline{2-6} 
                                        & Ours         & 1.76            & 2.09           & 1.65            & \textbf{1.59}   \\ \hline
\multirow{4}{*}{Background Consistency} & SVD-xt       & 0.92            & \textbf{0.97}  & \textbf{0.92}   & 0.89            \\ %\cline{2-6} 
                                        & Vista        & 0.92            & 0.96           & 0.91            & 0.89            \\ %\cline{2-6} 
                                        & StreamingT2V & 0.89            & 0.93           & 0.88            & 0.86            \\ %\cline{2-6} 
                                        & Ours         & \textbf{0.92}   & 0.94           & 0.91            & \textbf{0.91}   \\ \hline
\end{tabular}
\caption{Comparison of results for generating long-duration videos on NuScenes. Our method demonstrates superior performance in terms of FID, FVD, highlighting its ability to generate high-quality, consistent long-duration driving scenarios.}
\label{tab:long-term-comparison}
\end{table*}

\section{Additional Experiment}
\subsection{Additional Metrics on Long-term Generation}
To demonstrate the efficacy of our world model in generating videos of long duration, we compare our method with several other state-of-the-art video generation methods in terms of long-term generation, and we include more metrics such as MAWE\cite{streamingT2V} and background consistency\cite{vbench} in addition to FID\cite{FID} and FVD\cite{fvd}. We measure these results using the first 120 frames of generated video clips with anchor frames from NuScenes\cite{nuscenes} validation set. Furthermore, to show the stability and consistency of our method in generating evolving driving scenarios over long course of time, we compare the results of our methods and other state-of-the-art methods during different frame windows. In particular, for each method we sample three 40 frame video segments from three consecutive frame windows: 0-40 frame, 40-80 frame and 80-120, and compute the metrics on each of them, displaying the change of metrics over an evolving time course. In addition to FID and FVD, we further show results in MAWE and the background consistency. As illustrated in Tab~\ref{tab:long-term-comparison}, our model performs better than the other methods do by a large margin in terms of FID, FVD both over all frames and over different frame windows. Moreover, our method maintains a comparable results in MAWE and the background consistency with other state-of-the-art methods over all frames, and as time goes by our method progressively catch up and show better consistency and motion dynamics beyond 80 frames. This trend in MAWE and the background consistency is also shown in Fig~\ref{fig:evolve_addition}, which is consistent to our result with FID and FVD metrics. This result highlights our method's capability of generating high-quality, consistent and diverse videos in long duration.

\begin{figure}[t]
  \centering
  %\fbox{\rule{0pt}{2in} \rule{0.9\linewidth}{0pt}}
   \includegraphics[width=1.00\linewidth]{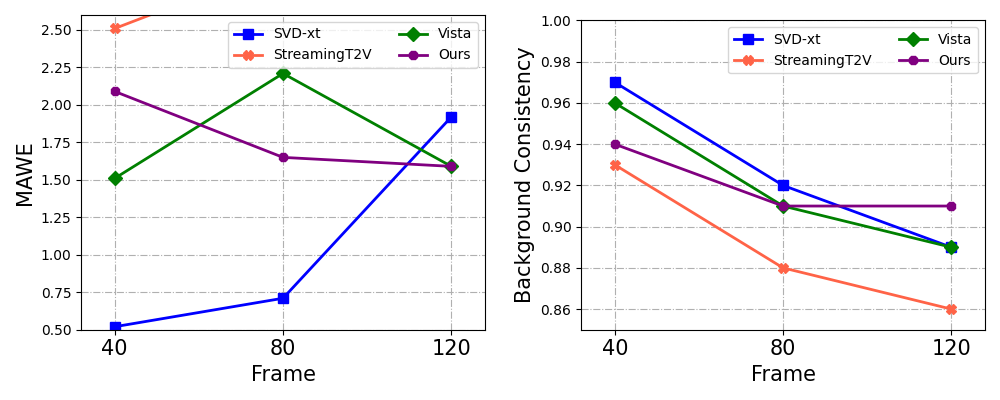}
   \caption{The curves of MAWE and Background Consistency as world models evolve with duration of time across different frames. Please note that MAWE yields a low value when videos are consistency and rich in motion, and the background consistency yields a high value close to 1.0 when videos are consistent in backgrounds. We measure MAWE and Background Consistency at frame 40, 80, 120, using the generated results of previous 40 frames at each time frame point.}
   \label{fig:evolve_addition}
\end{figure}

\begin{figure}[t]
  \centering
  %\fbox{\rule{0pt}{2in} \rule{0.9\linewidth}{0pt}}
   \includegraphics[width=1.00\linewidth]{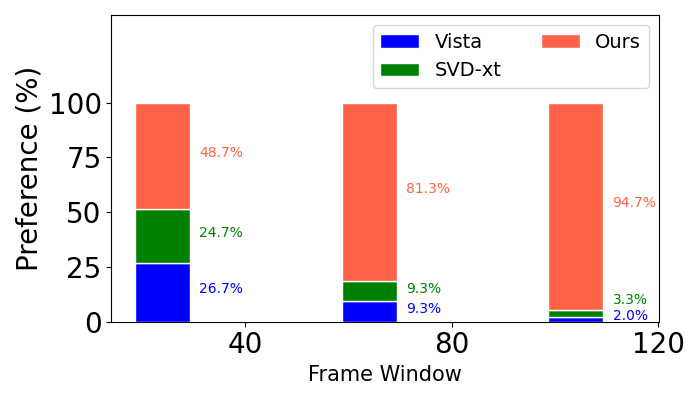}
   \caption{We collect human preference annotations from human annotators to evaluate the consistency and motion dynamics of generated videos by our method and two other state-of-the-art methods. This bar plot shows the percentage of human preferences at frame 40, 80, 120, using the generated results of previous 40 frames at each time frame point. As illustrated by the plot, our methods obtain most human preferences at all frame point, and gains more preference as the frame goes, showing the high consistency and rich motion dynamics of our methods at both short and long range generated videos.}
   \label{fig:huamn_eval}
\end{figure}

\subsection{Human Evaluation}
Automatic metrics such as FID\cite{FID} and FVD\cite{fvd} are well known for their inability to give concrete assessment of visual quality of simulated world scenarios \cite{video,genad,emu}. We therefore include a human evaluation for a more faithful assessment of our methods. We adopt a preference selection protocol, where we present to the human annotators the generated video clips of three methods including ours, SVD-xt\cite{svd} and Vista\cite{vista}, and we ask the human annotators to rank their preference of three generated results based on visual quality, consistency and motion dynamics. Moreover, to evaluate the long-term video quality, we again divide the generated videos into three segments based on frame windows of 0-40, 40-80 and 80-120, and perform human preference selection for all three segments. We adopt the scenes from NuScenes\cite{nuscenes} validation set, and for all three methods we use the same initial condition images, and resize the generated videos to a fixed resolution of 288x512 and stitch them side by side. We collect 450 human preference results out of 150 scenes of NuScenes validation sets and 3 different frame window segments. We calculate the percentage of top preferences of each method in Fig~\ref{fig:huamn_eval}, and it shows that our method outperforms others in all three frame windows and as frame number increases our method gains more popularity, which demonstrates the visual quality, consistency and motion dynamics InfinityDrive in long duration video generation.

\section{Discussion}
In this section we wish to help the reader get a thorough understanding of this paper by discussing topics that may raise concerns.
\subsection{Potential Applications}

\noindent \textbf{Synthetic Data Generation} InfinityDrive can be extended to surrounding views and more fine-grained controllability with moderate modifications\cite{magicdrive}, and serve as a foundational model to generate multi-view driving data with control conditions such as mapping layout and bounding boxes. Moreover, InfinityDrive can generate diverse minute-long videos of high resolution and quality, which are crucial for developing robust autonomous driving models. High resolution and quality means the synthetic dataset can faithfully reflect the real world environment, and the long duration enables the video to cover a much wider range of scenarios. For instance, the scenario of vehicle stopping and waiting for green light in a busy intersection may last from tens of seconds to even minutes, and can include many perceptual and planning challenges for autonomous driving agents. Scenario diversity allows systems to train on a wide range of conditions, including rare and challenging edge cases, improving robustness and adaptability. InfinityDrive can generate such crucial yet frequent scenes, while other state-of-the-art methods can not due to the long duration requirement\cite{streamingT2V,vista,genad}. This ability to infer synthetic data that both align with the real world environment and cover a diverse range of driving scenarios, indicates the potential of InfinityDrive to generate data for training autonomous driving models.

\noindent \textbf{Closed-Loop Testing Simulation}. 
Closed-loop simulating refers to a dynamic simulation process where the outputs or actions of a system being tested (e.g., an autonomous agent) directly influence the ongoing state and evolution of the simulated environment in real-time. InfinityDrive’s strengths in generating long-duration, diverse, and high-quality videos make it exceptionally suited for closed-loop simulation. Its ability to create temporally consistent extended scenarios ensures seamless testing over long periods, capturing the sustained performance of autonomous systems. The diversity of simulated environments, from varying weather conditions to complex traffic dynamics, exposes systems to a wide range of real-world challenges. High-fidelity rendering further enhances precise perception modeling, critical for object recognition and sensor integration. Together, these capabilities enable InfinityDrive to dynamically adapt simulations in response to agent actions, creating realistic, responsive environments ideal for evaluating and refining autonomous systems in complex, evolving scenarios.

\noindent \textbf{Closed-Loop Training Simulation}.Closed-Loop Training Simulation refers to a dynamic and interactive simulation framework where the outputs or actions of the system being trained directly influence the evolution of the simulated environment, forming a real-time feedback loop. This approach allows the system to learn and adapt in response to its interactions with a constantly changing environment. InfinityDrive plays a crucial role in this framework by leveraging its ability to generate diverse and high-quality simulations. One of its standout features is the capability to create multiple parallel worlds from the same initial conditions. This enables rapid exploration of various possible trajectories and outcomes, allowing the system to compare and evaluate different decision-making strategies. By identifying the most optimal predictions across these parallel scenarios. InfinityDrive can enhances the system's ability to generalize and perform reliably in real-world settings. This dynamic diversity ensures comprehensive training that accounts for both common and edge-case scenarios, ultimately leading to more robust and adaptive models.

\noindent \textbf{City-Level Simulated Cruising.} With its capabilities for long-term video generation, InfinityDrive could be further developed to incorporate real-world road structures and traffic flow information as prior knowledge. Such integration would enable the creation of city-scale simulations that unify perception, planning, and navigation. For example, by embedding OpenStreetMap data and traffic flow models, InfinityDrive could simulate realistic urban driving scenarios, including traffic jams, pedestrian crossings, and traffic light patterns. This would not only benefit autonomous vehicle testing but also urban planning and the development of advanced driver-assistance systems (ADAS). Furthermore, combining these simulations with generative AI techniques could allow city-level traffic optimization studies, enabling researchers to test and improve traffic management strategies without disrupting real-world systems.

\subsection{Future Work}
Given the constraints of workload, this paper primarily concentrates on tackling the challenge of generating temporally consistent, high-fidelity long-duration videos. As a result, our method presents opportunities for further enhancement and development in future work.

\noindent \textbf{Multi-View Generation.} The current implementation of InfinityDrive is limited to single camera view, specifically the frontal view. It can be potentially extended to support multi-view video generation through multi-view cross attention\cite{magicdrive}. 

\noindent \textbf{More Modalities for Control.} InfinityDrive currently uses textual prompts and condition images for controlling video generation, but finer control modalities are essential for more complex applications. Future work could include mapping layouts for road geometries, bounding boxes for traffic participants, and dynamic event triggers like traffic light changes or pedestrian movements. These enhancements would allow developers to create highly specific and structured scenarios, which are valuable for autonomous driving models. Introducing more control options would greatly expand InfinityDrive’s utility in generating realistic, scenario-specific data for training and validation

\noindent \textbf{Inference Acceleration.} Due to the large number of sampling steps required by the DDPM algorithm, and the inherently high computational cost of video generation tasks—owing to the simultaneous existence of temporal and spatial dimensions—a significant amount of computation is inevitably needed. Employing methods like Rectified Flow, consistency distillation, or traditional model compression techniques can alleviate this issue. These optimizations would enable real-time video generation, making InfinityDrive suitable for interactive simulations and large-scale data production. Accelerating inference would significantly enhance the practicality and scalability of InfinityDrive, allowing it to meet the growing demands of industries relying on synthetic video data.

\noindent \textbf{End-to-End Training.} InfinityDrive can enable integration with reinforcement learning pipelines to support end-to-end training of autonomous systems. By exposing models to diverse scenarios during training, it can improve the adaptability of autonomous systems to dynamic environments. InfinityDrive can create a true closed-loop training process. Its ability to generate diverse trajectories from the same starting point allows for exposure to a broad range of scenarios, helping systems learn to generalize effectively. This integration would be particularly impactful for training autonomous vehicles to handle edge cases and adapt to complex, evolving situations, ultimately enhancing system robustness and real-world performance.

% {
%     \small
%     \bibliographystyle{ieeenat_fullname}
%     \bibliography{main}
% }
